# Supplementary material for: Can Agents Infer Environment from Interaction? Evidence from Agentic Automata Learning
Source: arXiv:2606.16576 source file (2026-09-27)
Supplement: Supplementary file 1 [file 06_context_window_analysis.tex]

\section{Context Window Analysis}
\label{sec:context_window}

\begin{figure}[t]
    \centering
    \includegraphics[
        width=\columnwidth,
        height=6.2cm,
        keepaspectratio
    ]{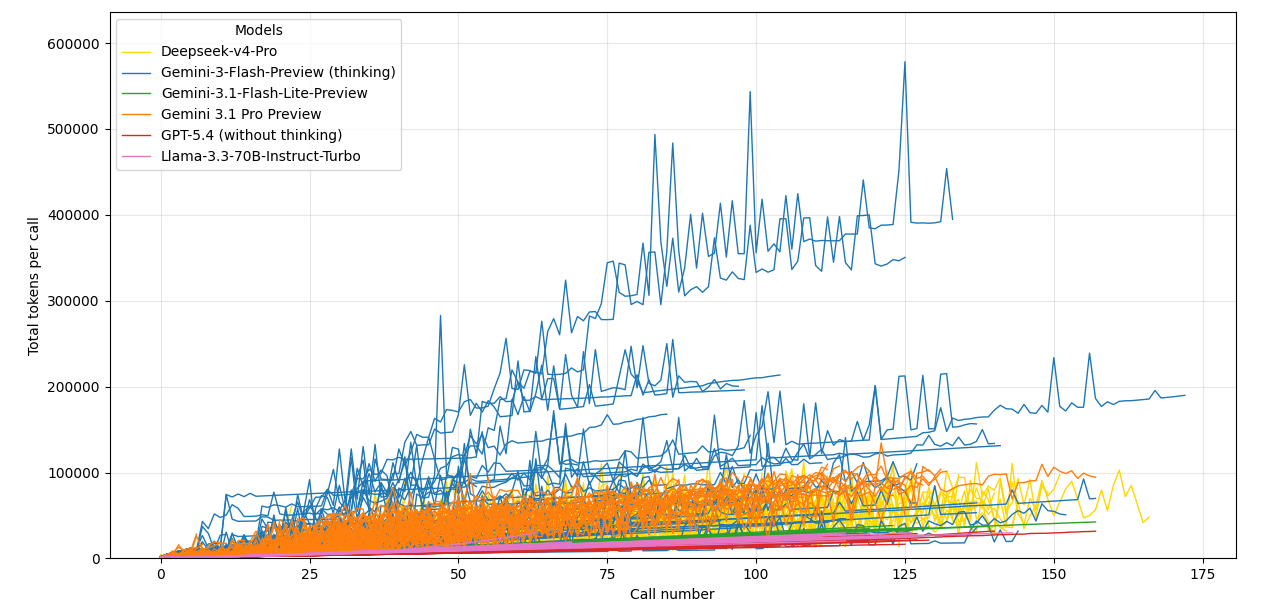}
    
    \caption{
    Context window size throughout interaction. Each line represents a single task instance, while colors correspond to different models. The figure shows how context size evolves across tool-call steps during task execution.
    }
    \label{fig:context_window_analysis}
\end{figure}
