# Supplementary material for: Can Agents Infer Environment from Interaction? Evidence from Agentic Automata Learning
Source: arXiv:2606.16576 source file (2026-09-27)
Supplement: Supplementary file 2 [file minimal_counterexample_information.tex]

\section{Why Minimal Counterexamples Provide Implicit Information}
\label{sec:minimal_counterexample_information}

A random counterexample provides only local information: it identifies a single word on which the hypothesis automaton and the target DFA disagree. In contrast, a minimal counterexample provides additional implicit information beyond the returned word itself. If the returned word is the shortest one on which the hypothesis and the target differ, then it follows that no shorter word distinguishes between them. Thus, minimality does not only identify a specific error, but also rules out an entire set of possible disagreements at shorter lengths. In addition, even when the model is not explicitly told that the returned counterexample is minimal, we estimate that repeated exposure during interaction to consistently short counterexamples may allow the model to infer that the oracle is returning the minimal counterexample, and to exploit the implicit information induced by this behavior.
